# Supplementary material for: Improving Fast Adversarial Training with Prior-Guided Knowledge
Source: arXiv:2304.00202 source file (2023-04-06)
Supplement: Supplementary file 1 [file appendix.tex]

\appendixpage
\begin{proof}

    The first part of the desired result can be proven using Jensen's inequality 
    \begin{equation}
        \left(\mathbb{E}_{\boldsymbol{\hat{\delta}}_{adv}\sim\boldsymbol{\Omega}}\Big[\big\|\boldsymbol{\hat{\delta}}_{adv}\big\|_2\Big]\right)^2\leq\mathbb{E}_{\boldsymbol{\hat{\delta}}_{adv}\sim\boldsymbol{\Omega}}\Big[\big\|\boldsymbol{\hat{\delta}}_{adv}\big\|^2_2\Big].
    \end{equation}
    In the following we focus on $\mathbb{E}_{\boldsymbol{\hat{\delta}}_{adv}\sim\boldsymbol{\Omega}}\Big[\|\boldsymbol{\hat{\delta}}_{adv}\|^2_2\Big]$. Denote
    \begin{equation}
        \boldsymbol{\nabla} = \nabla_{\mathbf{x}} \mathcal{L}(f(\mathbf{x}+\mathbf{\boldsymbol{\delta}_{pgi}}; \mathbf{w}), \mathbf{y}),
    \end{equation}
    we have
    \begin{equation}
        \label{eq:1}
        \begin{aligned}
            & & &\ \ \mathbb{E}_{\boldsymbol{\hat{\delta}}_{adv}\sim\boldsymbol{\Omega}}\Big[\|\boldsymbol{\hat{\delta}}_{adv}\|^2_2\Big]\\[5pt]
            & &=&\ \ \mathbb{E}_{\boldsymbol{\hat{\delta}}_{adv}}\Big[\big\|\Pi_{\boldsymbol{\Omega}}\big[\mathbf{\boldsymbol{\delta}_{pgi}}+\alpha\cdot\operatorname{sign}(\boldsymbol{\nabla})\big]\big\|^2_2\Big]\\[5pt]
            & &=&\ \ \sum_{i=1}^d \mathbb{E}_{\delta_{pgi}(i)}\Big[\Pi_{\boldsymbol{\Omega}}\big[\mathbf{\delta}_{pgi}(i)+\alpha\cdot\operatorname{sign}(\nabla_i)\big]^2\Big]\\[5pt]
            % & &=&\ \ d\cdot\mathbb{E}_{\delta_t(i)}\Big[\textbf{min}\Big\{|\delta_{t+1}(i)-\delta_{t}(i)|,\big|\mathbf{\delta}_t(i)+\alpha\cdot\operatorname{sign}(\nabla_i)\big|\Big\}^2\Big]\\[5pt]
            % & &=&\ \ d\cdot\mathbb{E}_{\delta_t(i)}\Big[\textbf{min}\Big\{|\delta_{t+1}(i)-\delta_{t}(i)|^2,\big(\mathbf{\delta}_t(i)+\alpha\cdot\operatorname{sign}(\nabla_i)\big)^2\Big\}\Big]\\[5pt]
            & &\leq&\ \ d\cdot\mathbb{E}_{\delta_{pgi}(i)}\Big[\textbf{min}\Big\{\frac{\epsilon^2}{d},\big(\mathbf{\delta}_{pgi}(i)+\alpha\cdot\operatorname{sign}(\nabla_i)\big)^2\Big\}\Big]\\[5pt]
            & &=&\ \ d\cdot\mathbb{E}_{r_i}\Bigg[\mathbb{E}_{\delta_{pgi}(i)}\Big[\textbf{min}\Big\{\frac{\epsilon^2}{d},\big(\mathbf{\delta}_{pgi}(i)+\alpha\cdot\operatorname{sign}(\nabla_i)\big)^2\Big\}\Big]\ \Bigg|\ \operatorname{sign}(\nabla_i)=r_i\Bigg],
        \end{aligned}
    \end{equation}
    where the last setp follows the low of total expectation as $r_i:=\operatorname{sign}(\nabla_i)$ is also a random variable depending on $\delta_t(i)$. 

    As $r_i$ is a binary random variable, $d$ is the feature dimension, and $\alpha<\epsilon$, it holds that
    \begin{equation*}
        \begin{aligned}
            & - \epsilon d^{-1/2} &>&\ \  -\epsilon + \alpha\\
            & \epsilon d^{-1/2} &<&\ \ \epsilon + \alpha,
        \end{aligned}
    \end{equation*}
    and we could separate the procedure into the following two cases:
    \begin{itemize}
        \item[(i)] $r_i=1$, the inner conditional expectation has the form:
        \begin{equation}
            \label{eq:2}
            \begin{aligned}
                & & &\ \ \int_{-\epsilon}^{\epsilon}\textbf{min}\left\{\frac{\epsilon^2}{d},(\delta_{pgi}(i)+\alpha)^2\right\}\frac{1}{2\epsilon}d\delta_{pgi}(i)\\[5pt]
                & &=&\ \ \frac{1}{2\epsilon}\int_{-\epsilon+\alpha}^{\epsilon+\alpha}\textbf{min}\left\{\frac{\epsilon^2}{d},x^2\right\}dx\\[5pt]
                & &=&\ \ \frac{1}{2\epsilon}\left(\int_{\epsilon d^{-1/2}}^{\epsilon+\alpha}\frac{\epsilon^2}{d}dx+\int_{-\epsilon d^{-1/2}}^{\epsilon d^{-1/2}}x^2dx + \int_{-\epsilon+\alpha}^{-\epsilon d^{-1/2}}\frac{\epsilon^2}{d}dx \right)\\[5pt]
                % & &=&\ \ \frac{\alpha^2}{2}+\frac{\epsilon^2}{3}-\frac{\alpha^3}{6\epsilon}.
                & &=&\ \ \frac{\epsilon}{2d}\left(2\epsilon-2\epsilon d^{-1/2}\right)+\frac{1}{3}\epsilon^2d^{3/2}\\[5pt]
                & &=&\ \
                \frac{\epsilon^2}{2d}-
                \frac{\epsilon^2}{d^{3/2}} +\frac{1}{3}\epsilon^2d^{-3/2}\\[5pt]
                % \frac{\epsilon^2}{4d}+\frac{\alpha\epsilon}{4d}+\frac{\epsilon^2}{48}-\frac{1}{6\epsilon}(\alpha-\epsilon)^3\\[5pt].
                % & &\leq&\ \ \frac{\epsilon^2}{2d} - \frac{\epsilon^2}{3d^{3/2}}+\frac{\epsilon^2}{6}
                & &\leq&\ \ \frac{\epsilon^2}{d}.
            \end{aligned}
        \end{equation}
        \item[(ii)] $r_i=-1$, the inner conditional expectation will be:
        \begin{equation}
            \label{eq:3}
            \begin{aligned}
                & & &\ \ \int_{-\epsilon}^{\epsilon}\textbf{min}\left\{\frac{\epsilon^2}{d},(\delta_{pgi}(i)-\alpha)^2\right\}\frac{1}{2\epsilon}d\delta_t(i)\\[5pt]
                & &=&\ \ \frac{1}{2\epsilon}\int_{-\epsilon-\alpha}^{\epsilon-\alpha}\textbf{min}\left\{\frac{\epsilon^2}{d},x^2\right\}dx\\[5pt]
                & &=&\ \ \frac{1}{2\epsilon}\left(\int_{\epsilon d^{-1/2}}^{\epsilon-\alpha}\frac{\epsilon^2}{d}dx+\int_{-\epsilon d^{-1/2}}^{\epsilon d^{-1/2}}x^2dx + \int_{-\epsilon-\alpha}^{-\epsilon d^{-1/2}}\frac{\epsilon^2}{d}dx \right)\\[5pt]
                % & &=&\ \ \frac{\alpha^2}{2}+\frac{\epsilon^2}{3}-\frac{\alpha^3}{6\epsilon}.
                & &=&\ \ \frac{\epsilon}{2d}\left(2\epsilon-2\epsilon d^{-1/2}\right)+\frac{1}{3}\epsilon^2d^{3/2}\\[5pt]
                & &=&\ \
                \frac{\epsilon^2}{2d}-
                \frac{\epsilon^2}{d^{3/2}} +\frac{1}{3}\epsilon^2d^{-3/2}\\[5pt]
                % \frac{\epsilon^2}{4d}+\frac{\alpha\epsilon}{4d}+\frac{\epsilon^2}{48}-\frac{1}{6\epsilon}(\alpha-\epsilon)^3\\[5pt].
                % & &\leq&\ \ \frac{\epsilon^2}{2d} - \frac{\epsilon^2}{3d^{3/2}}+\frac{\epsilon^2}{6}
                & &\leq&\ \ \frac{\epsilon^2}{d}.
                % & &\leq&\ \ \frac{\epsilon^2}{12}.        
            \end{aligned}
        \end{equation}
    \end{itemize}
    Combining \eqref{eq:2} and \eqref{eq:3} together with \eqref{eq:1}, we obtain
    \begin{equation*}
        \begin{aligned}
            & \mathbb{E}_{\boldsymbol{\hat{\delta}}_{adv}\sim\boldsymbol{\Omega}}\big[\|\boldsymbol{\hat{\delta}}_{adv}\|_2\big]&\leq&\ \ \sqrt{\ \mathbb{E}_{\boldsymbol{\hat{\delta}}_{adv}\sim\boldsymbol{\Omega}}\big[\|\boldsymbol{\hat{\delta}}_{adv}\|^2_2\big]}\\
            % & &\leq&\ \ \sqrt{\frac{3d^{1/2}+2+d^{3/2}}{6d}}\cdot\epsilon.
            & &\leq&\ \ \sqrt{\frac{1}{d}}\cdot\epsilon.
        \end{aligned}        
    \end{equation*}
\end{proof}
\noindent\textbf{Remark.} 
If $\boldsymbol{\Omega}$ is a bounded set like $ \boldsymbol{\Omega} = \big\{\boldsymbol{\hat{\delta}}_{adv}\ :\ \|\boldsymbol{\hat{\delta}}_{adv}-\boldsymbol{\delta}_{pgi}\|^2_2\leq{\epsilon}^{2}\big\}$, we can obtain the upper bound of the proposed method which is $\sqrt{\frac{1}{d}}\cdot\epsilon$, which is less than the bound $\sqrt{\frac{d}{3}}\cdot\epsilon$ of FGSM-RS  provided in \cite{andriushchenko2020understanding} when $ d \textgreater \sqrt{3}$. It requires that the prior-guided adversarial perturbation $\boldsymbol{\delta}_{pgi}$ is not far from the current adversarial perturbation  $\boldsymbol{\hat{\delta}}_{adv}$. Additionally, the value of $d$ represents the dimension of image data, which is typically much larger than 4.

% According to the transferability of adversarial examples, the prior-guided adversarial perturbation $\boldsymbol{\delta}_{pgi}$ and the current adversarial perturbation  $\boldsymbol{\hat{\delta}}_{adv}$ both exist in the same adversarial subspace. In this way, the prior-guided adversarial perturbation $\boldsymbol{\delta}_{pgi}$ is not far from the current adversarial perturbation  $\boldsymbol{\hat{\delta}}_{adv}$.

% By the monotonicity of the FGSM type methods \cite{dou2018mathematical}, we know that the bounded set $\boldsymbol{\Omega}$ will be shrinkage during the adversarial perturbation. It means that the proposed prior-guided adversarial initialization will conduct the more efficient step size than \cite{andriushchenko2020understanding}.

% \begin{equation}
%         \begin{aligned}
%               & & &\min_{\mathbf{w}} \mathbb{E}_{(\mathbf{x}, y) \sim \mathcal{D}}\left[\max_{\boldsymbol{\theta}}~\mathbb{E}_{ \mathbf{a} \sim p(\mathbf{a}| \mathbf{x};\boldsymbol{\theta})}~[\mathcal{L}_1(\mathbf{w},\boldsymbol{\theta})+ \alpha \mathcal{L}_2(\boldsymbol{\theta}) + \beta \mathcal{L}_3(\boldsymbol{\theta})]\right],
%         \end{aligned}
%         \label{eq:newAT_pro}
%     \end{equation}
